# Supplementary material for: The Robots are Here: Navigating the Generative AI Revolution in Computing Education
Source: arXiv:2310.00658 source file (2023-10-01)
Supplement: Supplementary file 1 [file instructor-guide.tex]

\section{Guide for instructions}
